# Supplementary material for: Relaxed Paxos: Quorum Intersection Revisited (Again)
Source: arXiv:2203.03058 source file (2022-03-06)
Supplement: Supplementary file 1 [file additional_configs.tex]

\begin{figure}
  \centering
  \begin{footnotesize}
    \begin{subfigure}[b]{0.45\textwidth}
      \centering
      \begin{tabular}{ |l|l|}
        \hline
        \boldmath$i=$ & \boldmath$Q_i=$ \\
        \hline
        $0, 1, \dots$ & $\{\{S0,S1,S2\}, \{S0,S1,S3\},$ \\
        & $\{S0,S2,S3\}, \{S1,S2,S3\} \}$ \\
         \hline
      \end{tabular}
      \caption{}
      \label{fig:example_configs/4s_intersecting}
    \end{subfigure}
    \begin{subfigure}[b]{0.45\textwidth}
      \centering
      \begin{tabular}{ |l|l| }
        \hline
        \boldmath$i=$ & \boldmath$Q_i=$ \\
        \hline
        $0, 1, 2$ & $\{\{S0,S1,S2\}\}$ \\
        $3, 4, \dots $ & $\{\{S0,S1\}, \{S0,S2\}, \{S1,S2\}\}$ \\
        \hline
      \end{tabular}
      \caption{}
      \label{fig:add_example_configs/allin}
    \end{subfigure}
    \begin{subfigure}[b]{0.45\textwidth}
    \centering
    \begin{tabular}{ |l|l|}
      \hline
      \boldmath$i=$ & \boldmath$Q_i=$ \\
      \hline
      $0$ & $\{\{S0,S1\}\}$ \\
      $1, 2, \dots $ & $\{\{S0,S1\}, \{S0,S2\}, \{S1,S2\}\}$ \\
      \hline
    \end{tabular}
    \caption{}
    \label{fig:add_example_configs/fixedmaj}
    \end{subfigure}
    \begin{subfigure}[b]{0.45\textwidth}
      \centering
      \begin{tabular}{ |l|l|}
        \hline
        \boldmath$i=$ & \boldmath$Q_i=$\\
        \hline
        $0, 1, \dots, 10$ & $\{\{S0,S1\}, \{S0,S2\}, \{S1,S2\}\}$  \\
        $11, \dots$ & $\{\{S3,S4\}, \{S3,S5\}, \{S4,S5\}\}$  \\
        \hline
      \end{tabular}
      \caption{}
      \label{fig:add_example_configs/reconfig}
    \end{subfigure}
  \caption{Additional sample configurations.}
  \label{fig:add_example_configs}
  \end{footnotesize}
\end{figure}
